# Supplementary material for: LM vs LM: Detecting Factual Errors via Cross Examination
Source: arXiv:2305.13281 source file (2023-05-22)
Supplement: Supplementary file 1 [file 0C_appendix.tex]

\section{Cross Examination Algorithm}

Here we describe our method via pseudo-code. 

\begin{algorithm}[t]
\caption{Cross Examination}
\textbf{Input:} A claim $C$ generated by \claimLLM{} \\
\textbf{Output:} Correct / Incorrect
\label{alg:cross_examination}
\begin{algorithmic}

\State $Report \gets ""$
\State $Q \gets \examinerLLM{}(\mathcal{P}_{setup}, C)$
\State $R_{curr} \gets \claimLLM{}(C, Q)$
\State $Report \gets Report + Q + R_{curr}$
\While{$\examinerLLM{}(\mathcal{P}_{follow-up}, R)$ is ``Yes''}
\State $Q \gets \examinerLLM{}(\mathcal{P}_{follow-up}, R)$
\State $R_{prev} \gets R_{curr}$
\State $R_{curr} \gets \claimLLM{}(R_{prev}, Q)$
\State $Report \gets Report + Q + R_{curr}$
\EndWhile
\State \Return $\examinerLLM{}(\mathcal{P}_{decision}, C, Report)$

\end{algorithmic}
\end{algorithm}
